# Supplementary material for: Boosting Language Models Reasoning with Chain-of-Knowledge Prompting
Source: arXiv:2306.06427 source file (2024-06-03)
Supplement: Supplementary file 1 [file appendix-io-examples-coin.tex]

% \begingroup
\begin{table}
    \centering
    \small
    \begin{tabular}{p{\linewidth}}
        \toprule
        \textbf{\textsc{Question:}} A coin is heads up. Andree flips the coin. Audrie does not flip the coin. Is the coin still heads up?  \\
        \textbf{\textsc{Model Answer \color{ForestGreen}{(CORRECT)}:}} The coin was flipped by Andree. So the coin was flipped 1 time, which is an odd number. The coin started heads up, so after an odd number of flips, it will be tails up. So the answer is no. \color{ForestGreen}{\checkmark} \\
        \midrule
        \textbf{\textsc{Question:}} A coin is heads up. Kristian does not flip the coin. Dallas does not flip the coin. Is the coin still heads up? \\
        \textbf{\textsc{Model Answer \color{BrickRed}{(INCORRECT)}:}} The coin {\color{BrickRed} was flipped by Kristian}. So the coin was flipped 1 time, which is an odd number. The coin started heads up, so after an odd number of flips, it will be tails up. So the answer is no. \color{BrickRed}{\xmark} \\
        \bottomrule
    \end{tabular}
    \caption{
    Examples of correct and incorrect chains of thought produced by \sqs{Model Name} on the coinflip task.
    }
    \label{tab:appendix-coin-examples}
\end{table}
% \endgroup
