# Supplementary material for: Boosting Language Models Reasoning with Chain-of-Knowledge Prompting
Source: arXiv:2306.06427 source file (2024-06-03)
Supplement: Supplementary file 2 [file appendix-io-examples-letters.tex]

\begingroup
\begin{table}[h]
    \centering
    \small
    \begin{tabular}{p{\linewidth}}
        \toprule
        \textbf{\textsc{Question:}} Take the last letters of the words in ``Waldo Schmidt'' and concatenate them. \\
        \textbf{\textsc{Model Answer \color{ForestGreen}{(CORRECT)}:}} The last letter of ``Waldo'' is ``o''. The last letter of ``Schmidt'' is ``t''. Concatenating them is ``ot''. So the answer is ot. \color{ForestGreen}{\checkmark} \\
        \midrule
        \textbf{\textsc{Question:}} Take the last letters of the words in ``Daniel Friedman'' and concatenate them. \\
        \textbf{\textsc{Model Answer \color{BrickRed}{(INCORRECT)}:}} The last letter of ``Daniel'' is ``l''. The {\color{BrickRed} last letter of ``Friedman'' is ``m''.} Concatenating them is ``lm''. So the answer is lm. \color{BrickRed}{\xmark} \\
        \bottomrule
    \end{tabular}
    \caption{
    Examples of correct and incorrect chains of thought produced by \sqs{Model Name} on the letter concatenation task.
    }
    \label{tab:appendix-letter-examples}
\end{table}
\endgroup
