# Supplementary material for: Boosting Language Models Reasoning with Chain-of-Knowledge Prompting
Source: arXiv:2306.06427 source file (2024-06-03)
Supplement: Supplementary file 3 [file appendix-knowledge-bases.tex]

\section{Knowledge Bases}
